# Supplementary material for: Fractal basin geometry and the limits to predictability and reproducibility in deep learning
Source: arXiv:2510.05606 ancillary file (2026-11-20)
Supplement: Supplementary file 1 [file Supplementary_Information.pdf]

# Supplementary information for "Riddled basin geometry sets fundamental limits to predictability and reproducibility in deep learning"

Andrew Ly[1] and Pulin Gong[1*]

[1]School of Physics, University of Sydney, Sydney, NSW, Australia.

*Corresponding author(s). E-mail(s): pulin.gong@sydney.edu.au;

## 1 Mathematical description of riddling

The attractors of a dynamical system have fundamental bearing upon questions of long-term behavior. To introduce the theoretical conditions for riddled basins, we adopt a measure-theoretical definition of an attractor [1]. Consider a dynamical system whose time dependence is generated by the iteration of a map $\Phi : \mathbb{R}^d \to \mathbb{R}^d$. Suppose there exists an invariant set $A \subset \mathbb{R}^d$, such that $\Phi^t(A) \subset A$ for all $t$. The basin of attraction of $A$ is $\beta(A) := \{\boldsymbol{\theta} \in \mathbb{R}^d \mid \omega(\boldsymbol{\theta}) \subset A\}$, where the $\omega$-limit set $\omega(\boldsymbol{\theta}) := \cap_{t>0}\overline{\{\Phi^s(\boldsymbol{\theta}_0) \mid s > t\}}$ is the set of accumulation points of the trajectory $\Phi^t(\boldsymbol{\theta}_0)$ as $t \to \infty$. That is, $\beta(A)$ contains all points that accumulate in $A$. The invariant set $A$ is a Milnor attractor if $l(\beta(A)) > 0$ and $l(\beta(A) \setminus \beta(A')) > 0$ for any proper compact subset $A' \subset A$, where $l$ is the $d$-dimensional Lebesgue measure. In contrast to other definitions of an attractor, the basin of a Milnor attractor need not contain an open neighborhood of the attractor itself. Milnor attractors are essential for the formulation of riddled basins, as riddling can occur even arbitrarily close to the attractor, violating classical notions of Lyapunov stability. A basin of attraction $\beta(A)$ is riddled if for all $\boldsymbol{\theta} \in \beta(A)$ and $\delta > 0$ we have $l(B_\delta(\boldsymbol{\theta}) \cap \beta(A)^c) > 0$, where $B_\delta(\boldsymbol{\theta})$ denotes the $\delta$-neighborhood of $\boldsymbol{\theta}$ [2]. Thus any initialization attracted to $A$ is arbitrarily close to another initialization leading to a different attractor.

## 2 Regimes of riddling

At small learning rates, there is a periodic attractor in the invariant subspace $\mathcal{P}_+$. For example, at $\eta = 1$ there is a period-2 attractor whose periodic points are $(0.2049, 0.2049, 0.9554, 0.9554)$ and $(1.748, 1.748, 2.117, 2.117)$ approximately. When such a periodic attractor coexists with a non-attracting chaotic saddle, pseudo-riddling occurs [3, 4]: the basin of attraction comprises both riddled and non-riddled components (see Extended Data Fig. 5b). Note that the presence of a transversely unstable

periodic orbit embedded in the chaotic saddle is a necessary condition for pseudo-riddling. At very small learning rates (e.g., $\eta = 0.1$), where all periodic orbits are transversely stable, riddling is absent (see Extended Data Fig. 5a). Transverse stability weakens as the learning rate increases [5]. The point at which a periodic orbit becomes transversely unstable is the riddling bifurcation that marks the onset of pseudo-riddling.

At sufficiently large learning rates, the chaotic attractor in the invariant subspace $\mathcal{P}_+$ undergoes a blowout bifurcation, losing transverse stability [6]. This critical point coincides with the infinite-time transverse Lyapunov exponent becoming positive. After blowout, all initializations off the subspace will eventually move away. Nonetheless, initializations starting near the invariant subspace can experience an extremely long chaotic transient, especially close to the critical point. Because a chaotic transient prior to escape is indistinguishable from a chaotic attractor over finite training horizons (training time is always finite), the time-dependent basin of a chaotic transient is physically meaningful [7]. The basin of the chaotic transient at $\eta = 3$ (see Extended Data Fig. 5d) is riddled with divergent initializations. The Lebesgue measure of this time-dependent basin decreases to zero as training duration increases.

## 3 Unpredictable divergence of a long chaotic transient

The uncomputability of neural network training dynamics implies the existence of arbitrarily long chaotic transients with sudden, unpredictable divergences. We observe such a divergence in the trajectory used to represent the chaotic attractor in Fig. 2a of the main text. It diverges after approximately $9.4 \times 10^4$ epochs of intermittent switching between the two regions of the chaotic attractor (Fig. S1a-b). The long chaotic transient is governed by the complex gradient vector field closer to the origin (Fig. S1e). A sudden burst in $\boldsymbol{\theta} \cdot \mathbf{e}_1$ takes the trajectory far from the origin (Fig. S1c). Figure S1f shows that the global geometry of the loss function is a paraboloid with significantly larger curvature in the $\mathbf{e}_2$ direction compared to the $\mathbf{e}_1$ direction. As a result, the trajectory diverges in a direction approximately parallel to $\mathbf{e}_2$. The divergence rate is governed by the curvature of $L(\boldsymbol{\theta})$ along the diverging path. By least squares regression in Fig. S1d, $|\boldsymbol{\theta}_t \cdot \mathbf{e}_2| \sim \exp(t/t_c)$ with characteristic time $t_c = 2.466303467(5)$ epochs. Assuming a globally quadratic $L(\boldsymbol{\theta})$ with directional curvature $\lambda = \mathbf{e}_2^\top \mathbf{H} \mathbf{e}_2$, we predict the scaling $|\boldsymbol{\theta}_t \cdot \mathbf{e}_2| \sim (\eta - \lambda)^t$. Based on the estimated characteristic time, $\lambda = \eta - \exp(1/t_c) = 1.000000001(1)$. Indeed, by least squares regression, the quadratic cross-section of $L(\boldsymbol{\theta})$ in Fig. S1g has Hessian $\lambda = 0.9999999999999923(7)$, consistent with the prediction. In summary, this provides a concrete instance of uncomputable behavior: proximity to an attractor does not guarantee convergence.

## 4 Fractality in hyperparameter space

Recent findings [8] show that the boundary of neural network trainability, separating convergence and divergence in hyperparameter space, is fractal. Moreover, the best-performing hyperparameters tend to lie near this boundary. These two results have practical implications for hyperparameter optimization, which is within the remit of the meta-learning paradigm (i.e., learning-to-learn) [9]. They imply that hyperparameter optimization occurs within a space whose fractality fundamentally undermines the stability of the process. In this section, we explain these phenomena. To accomplish this, we emulate the experiments in [8] by training our minimal model with

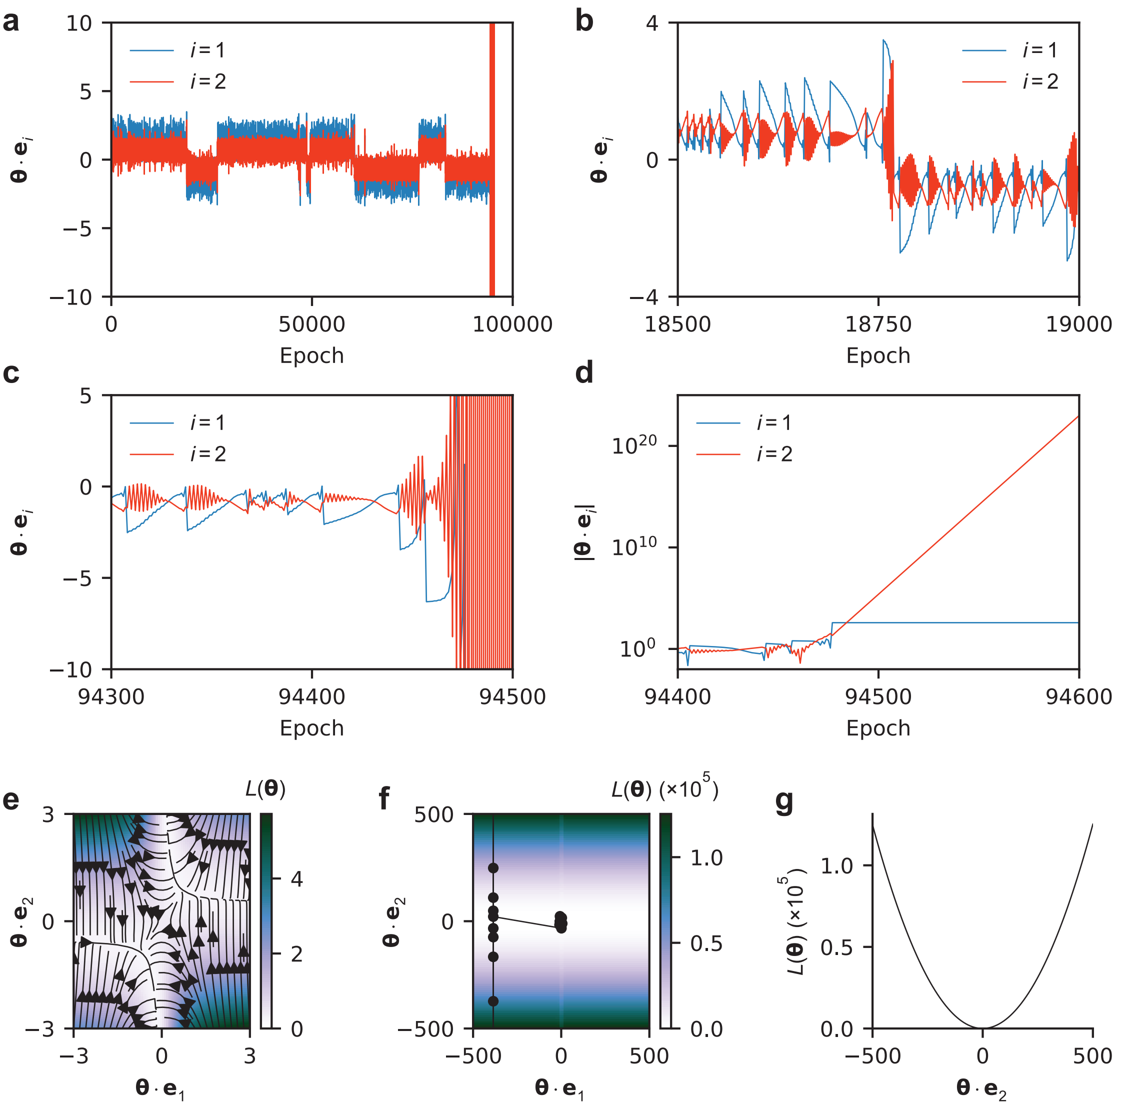


**Fig. S1 The unpredictable divergence of a long chaotic transient.** The trajectory used to visualize the chaotic attractor in Fig. 2a of the main text resides in $\mathcal{P}_+$, which has orthonormal basis vectors $\mathbf{e}_1 = (1, 1, 0, 0)/\sqrt{2}$ and $\mathbf{e}_2 = (0, 0, 1, 1)/\sqrt{2}$. **a,** The coordinates of the trajectory with respect to the basis of $\mathcal{P}_+$. **b,** Magnification of the intermittent switching behavior. **c,** Magnification of the sudden divergence. **d,** The magnitude of $\boldsymbol{\theta} \cdot \mathbf{e}_2$ diverges exponentially while $\boldsymbol{\theta} \cdot \mathbf{e}_1$ remains constant. **e,** Visualization of the loss function $L(\boldsymbol{\theta})$ in the vicinity of the chaotic attractor. Here the gradient vector field (black), $\nabla_{\boldsymbol{\theta}} L(\boldsymbol{\theta})$, is complex. **f,** Expanded view of the loss function, $L(\boldsymbol{\theta})$. The trajectory (black) diverges in the $\mathbf{e}_2$ direction. **g,** The vertical cross-section of $L(\boldsymbol{\theta})$ along the diverging path.

layer-specific learning rates $\eta^{(1)}$ and $\eta^{(2)}$. We visualize the training outcome in hyperparameter space for neural networks initialized at $(\boldsymbol{\theta} \cdot \mathbf{e}_{\parallel}, \boldsymbol{\theta} \cdot \mathbf{e}_{\perp}) = (0.539, 1.819)$, marked by the white cross in Fig. 1 of the main text (Fig. S2). The various phases of riddling in parameter space are discernible. For instance, there is no riddling at small $\eta$, basins of $\mathcal{P}_\pm$ are intermingled at around $\eta = 2.5$ (Fig. S2b), and basins are riddled with divergence at larger $\eta$. Moreover, the boundary separating convergence (blue and orange) and divergence (white) is indeed fractal.

To explain the fractality of this boundary, we first illustrate two generic mechanisms by which a fixed initialization transitions from convergence to divergence: (1) Hyperwedges (Extended Data Fig. 2) can bend towards different outcomes depending on the

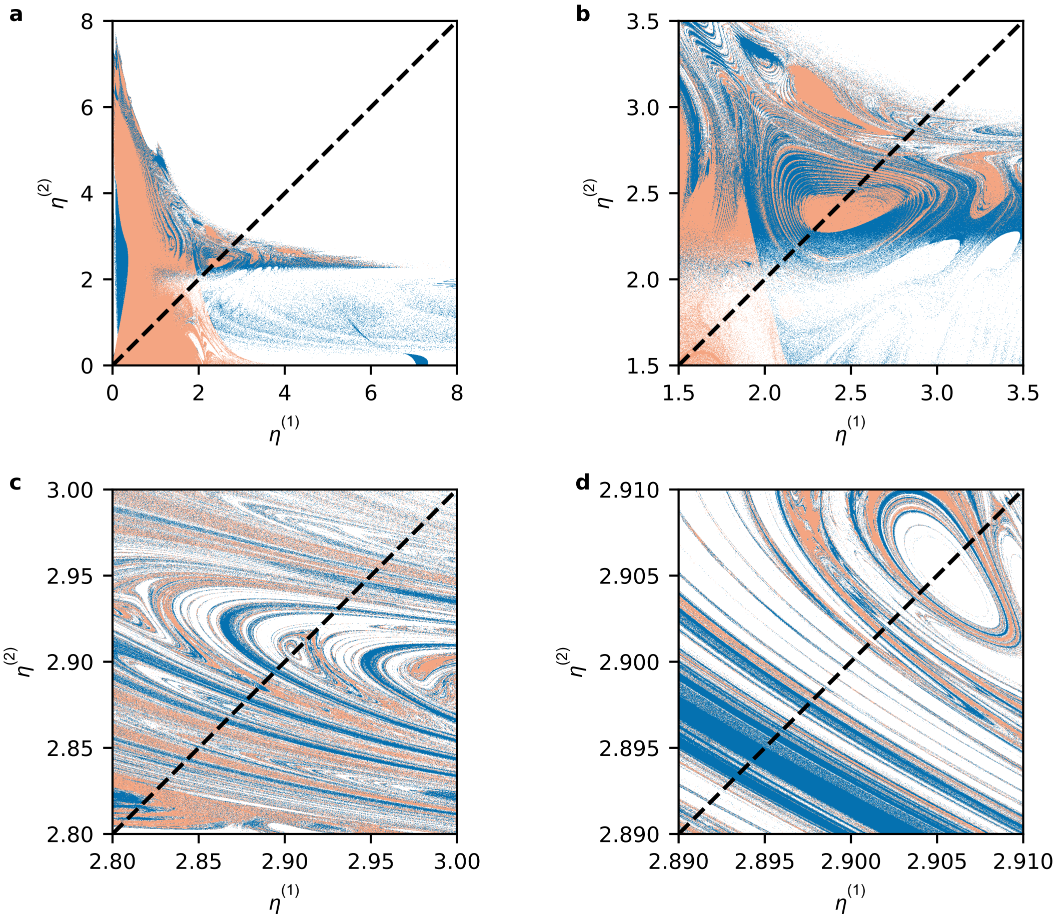


**Fig. S2 Destination map in hyperparameter space. a,** Training outcomes for the minimal model initialized at the white cross in Fig. 1 of the main text, $(\boldsymbol{\theta} \cdot \mathbf{e}_{\|}, \boldsymbol{\theta} \cdot \mathbf{e}_{\perp}) = (0.539, 1.819)$, is determined on a $1024 \times 1024$ grids over layer-specific learning rates, $\eta^{(1)}$ and $\eta^{(2)}$. Initializations converging to $\mathcal{P}_{+}$, $\mathcal{P}_{-}$ and infinity are colored blue, orange and white, respectively. The dashed line represents $\eta^{(1)} = \eta^{(2)}$, which applies to all neural networks in the main text. **b,** Magnification about $\eta^{(1)} = \eta^{(2)} = 2.5$. **c,** Magnification about $\eta^{(1)} = \eta^{(2)} = 2.9$, which is at the boundary of neural network trainability. **d,** Further 10-times magnification about $\eta^{(1)} = \eta^{(2)} = 2.9$.

destination of a heteroclinic trajectory. If a hyperwedge no longer intersects another invariant subspace (e.g., due to its sufficiently weakened transverse stability), and is instead diverted to infinity, then initializations caught in the hyperwedge will diverge. In this case, the basin is riddled with divergence (see e.g., Extended Data Fig. 5d). (2) If the learning rate exceeds the stability threshold of the parabolic loss function restricted to the invariant subspace $\mathcal{P}$ (i.e., $\eta > 2/\lambda$ where $\lambda$ is the largest curvature of the paraboloid), then infinity is an attractor on $\mathcal{P}$. As a result, initializations in $\mathcal{P}$ with large norms, as well as its pre-iterates with potentially small norms, will diverge. If this diverging trajectory has stable directions, then it can carry a volume of nearby initializations towards infinity as well. The suddenly diverging trajectory in Fig. S1 is an example of this situation.

These mechanisms determine the boundary separating convergence and divergence. For a given initialization, this hyperparameter-space boundary coincides exactly with the set of hyperparameters at which the boundary separating convergence and divergence in parameter space passes over that initialization. Since the parameter-space

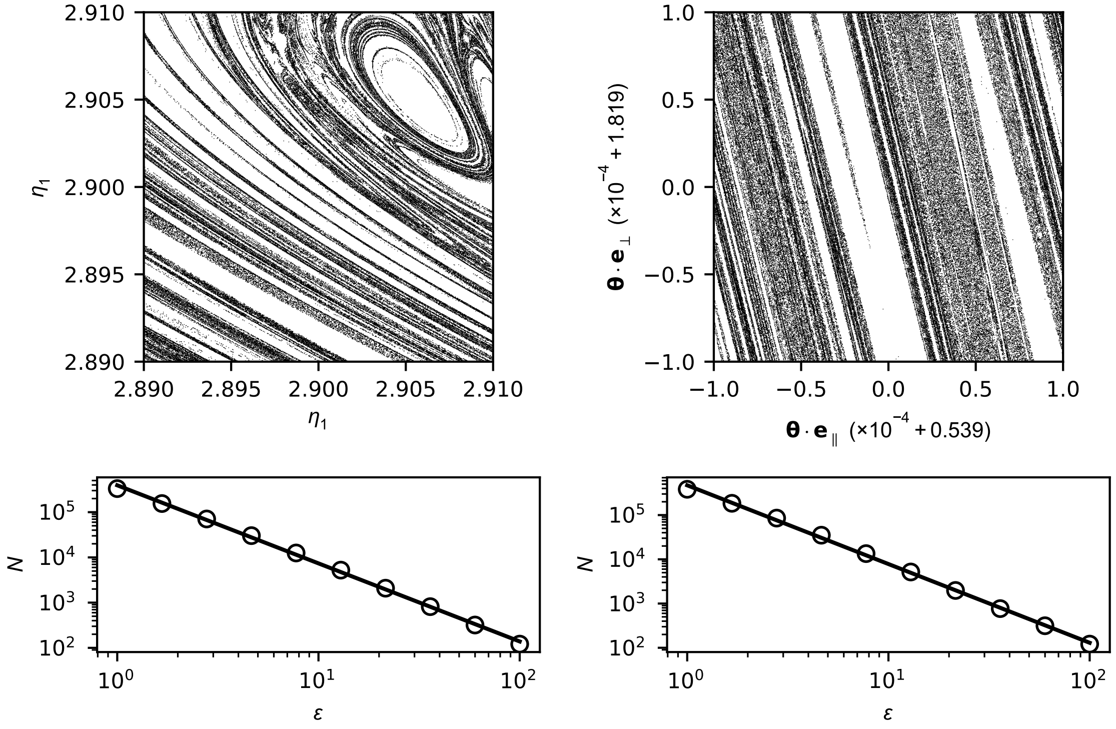


**Fig. S3 Fractal analysis of the boundary of network trainability. a,** The boundary of network trainability (black) is determined from the destination map in hyperparameter space (Fig. S2d). White points are in the interior of a basin. **b,** Same as (**a**), except in parameter space in the vicinity of the initialization $(\boldsymbol{\theta} \cdot \mathbf{e}_\parallel, \boldsymbol{\theta} \cdot \mathbf{e}_\perp) = (0.539, 1.819)$ at $\eta^{(1)} = \eta^{(2)} = 2.9$. **c,** Box counting for the boundary in hyperparameter space shows a fractal dimension of $d_{hp} = 1.73 \pm 0.02$. **d,** Box counting for the boundary in parameter space shows a fractal dimension of $d_p = 1.78 \pm 0.02$.

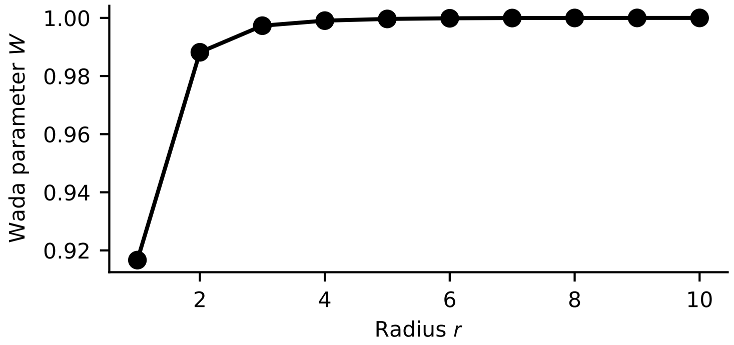


**Fig. S4 Wada property in hyperparameter space.** The Wada parameter $W$, which is the fraction of boundary points that exhibit the Wada property, is calculated from Fig. S2c using the merging method [11]. The method converges to show full Wada property with fattening radius $r = 9$.

boundary is fractal, the hyperparameter-space boundary is also fractal (Fig. S3(a-b)). Their (box-counting) fractal dimensions are similar: $d_p = 1.78 \pm 0.02$ and $d_p = 1.73 \pm 0.02$, respectively. We note that these fractal dimensions imply scaling laws for the predictability of divergence, as measured by the uncertainty exponent [10]. Specifically, the uncertainty exponents are $\phi_{\mathrm{p}} = 2 - d_{\mathrm{p}} = 0.22 \pm 0.02$ and $\phi_{\mathrm{hp}} = 2 - d_{\mathrm{hp}} = 0.27 \pm 0.02$. Thus, whether training converges or diverges is also sensitive to the configuration.

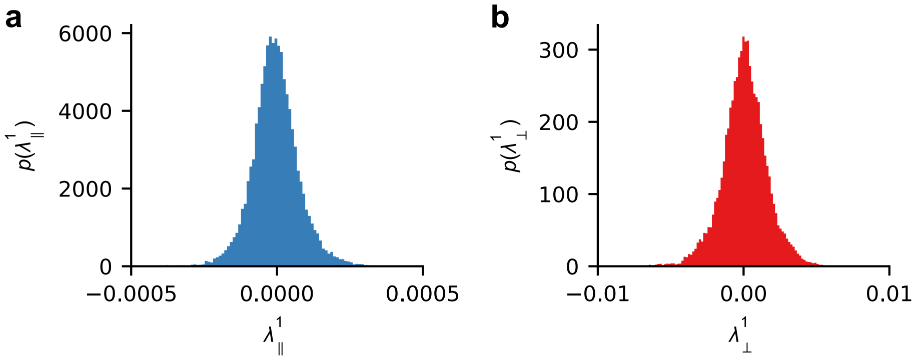


**Fig. S5 Local Lyapunov exponents.** Temporal distribution of local Lyapunov exponents across 50 epochs of training from the projection of the final state of the trajectory in Fig. 4a of the main text onto the invariant subspace. **a,** Maximal longitudinal exponent $\lambda_{\parallel}^1$. **b,** Maximal transverse exponent $\lambda_{\perp}^1$.

It is interesting to note that the hyperparameter-space basins near the boundary of neural network trainability (Fig. S2c-d) strongly resemble Wada basins [12]. A basin exhibits the Wada property if any point on its boundary is on the boundary of at least two other basins. We test the Wada property using the merging method [11] on Fig. S2c. The Wada parameter $W$, which represents the fraction of boundary points that exhibit the Wada property, quickly converges to $W = 1$ as the fattening radius $r$ increases. This is strong evidence that, in the vicinity of the convergence-divergence boundary, the basins in hyperparameter space are Wada. The Wada property places the predictability of the outcome in this region of hyperparameter space between fractal basins and riddled basins. In other words, there are pockets of training configurations in hyperparameter space, close to the boundary of trainability, whose outcomes are robust to sufficiently small perturbations (i.e., weaker than riddling). However, if a perturbation does change the outcome, then it is uncertain to which outcome (i.e., stronger than typical fractality). Note that at hyperparameters exhibiting Wada geometry, the corresponding parameter space contains a basin riddled with diverging initializations (see Extended Data Fig. 5d).

## 5 Local Lyapunov exponents of the deep neural network

We compute the local Lyapunov exponents (i.e., finite-time Lyapunov exponents $\lambda^T$ with $T = 1$) using the treppen-iteration algorithm with rectangular $\mathbf{Q}^0 = \big(\mathbf{e}_{\parallel}\ \mathbf{e}_{\perp}\big)$, where $\mathbf{e}_{\parallel}$ and $\mathbf{e}_{\perp}$ are longitudinal and transverse random orthonormal vectors (see equations (9-11) in Methods). Specifically, we accumulate local Lyapunov exponents starting from the final state of the trajectory in Fig. 4a of the main text projected onto the invariant subspace. We choose $\mathbf{e}_{\parallel}$ and $\mathbf{e}_{\perp}$ identical to those in Fig. 4b-d of the main text. Figure S5 shows the distribution of local Lyapunov exponents. The presence of positive longitudinal exponents indicates local instability, forming tentative evidence for chaotic behavior. Rigorous determination that the attractor in the invariant subspace is chaotic requires calculation of the infinite-time exponent, which is the time-average of the local exponents, if it converges. However, we observe that the empirical measure converges extremely slowly to the natural measure of the attractor due to the high dimensionality of the system. This difficulty prevents us from verifying all mathematically sufficient conditions for riddling in the deep neural network. The lower-dimensional minimal model avoids this issue. Similarly, positive fluctuations of the transverse exponent suggest that, if there is a chaotic attractor,

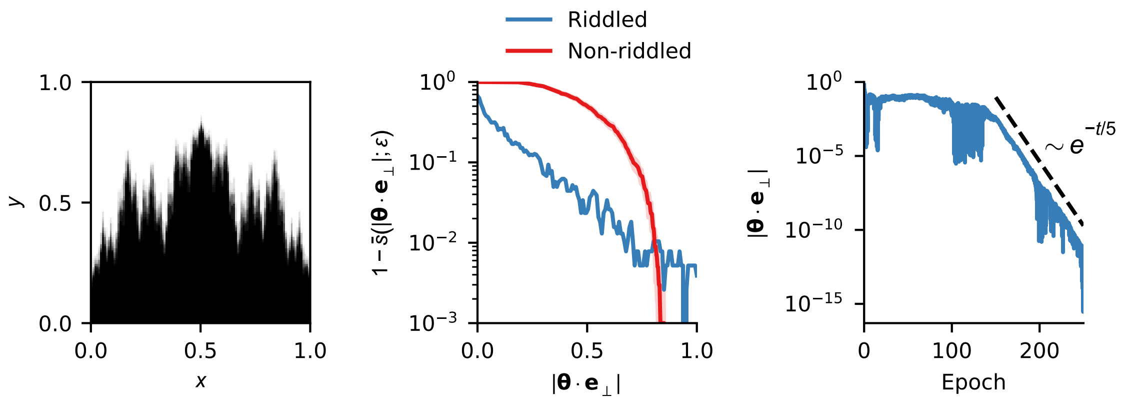


**Fig. S6 Riddling mechanism for critical learning periods. a,** Fractal but non-riddled basin generated from equations S1 and S2. Black and white represent initializations converging to $y = 0$ and $y = 1$, respectively. **b,** Comparison of the sensitivity metric $\bar{s}(|\boldsymbol{\theta}\cdot\mathbf{e}_\perp|;\varepsilon)$ for the non-riddled basin in (**a**) and the riddled basin in Fig. 4 of the main text. While $\bar{s}(|\boldsymbol{\theta}\cdot\mathbf{e}_\perp|;\varepsilon)$ vanishes at sufficiently small $|\boldsymbol{\theta}\cdot\mathbf{e}_\perp|$ in the former, it does not in the latter. **c,** Evolution of the transverse component $|\boldsymbol{\theta}\cdot\mathbf{e}_\perp|$ over 250 training epochs of the VGG-12 network. After an early period, the network converges exponentially to the invariant subspace.

its transverse stability would be weakened by the presence of transversely unstable atypical trajectories, sufficient for its basin to be riddled.

## 6 Riddling mechanism for critical learning period

We demonstrate a riddling mechanism for critical learning periods in neural network training [13, 14]. In particular, we show that a reduced but non-vanishing sensitivity to perturbations observed at later stages of training is explained by riddled basins. As a control, we illustrate that this is not possible for typical non-riddled basins.

To compare with the riddled basins of neural network training, we consider the following dynamical system that generates a representative non-riddled basin:

$$x_{t+1} = \lambda_x x_t \pmod 1 \tag{S1}$$

$$y_{t+1} = \frac{1}{\pi}\left[\tan^{-1}\left(\lambda_y \tan\left(\pi y_t - \frac{\pi}{2}\right)\right) + \cos(2\pi x_t) + \frac{\pi}{2}\right], \tag{S2}$$

where $\boldsymbol{\theta} = (x, y) \in [0,1]\times[0,1]$ and $\lambda_x, \lambda_y$ are analogous to parameters and hyperparameters, respectively. Specifically, $\lambda_x = 3$ and $\lambda_y = 1.5$. An equivalent two-dimensional map under the transformation $\tan\left(\pi\left(y - \frac{1}{2}\right)\right) \mapsto y$ has been studied previously [15]. We have rescaled the coordinates to have a finite domain, such that the Euclidean distances to the attractors at $y = 0$ and $y = 1$ are finite (in contrast to attractors at $y = \pm\infty$). Their basins of attraction are visualized in Fig. S6a, showing fractal but non-riddled structure.

As explained in the main text, the sensitivity of the learning process to perturbations is related to the probability that a point in the neighborhood of the network state belongs to a competing basin. Based on this geometric perspective, we introduce a sensitivity metric $s(\boldsymbol{\theta}, \varepsilon)$ defined as the fraction of the $\varepsilon$-hypercube centered at $\boldsymbol{\theta}$ occupied by a competing basin. To understand the critical learning period, we examine how this metric evolves as the network state progresses towards an attractor. Thus, we

determine the average sensitivity $\bar{s}(|\boldsymbol{\theta} \cdot \mathbf{e}_{\perp}|; \varepsilon)$ across points of varying distance from the attractor as measured by the transverse component $|\boldsymbol{\theta} \cdot \mathbf{e}_{\perp}|$ (Fig. S6b). For the VGG-12 network, we use the same $\mathbf{e}_{\perp}$ as Fig. 4 in the main text. For the dynamical system, we use $\mathbf{e}_{\perp} = (0, 1)$ such that $|\boldsymbol{\theta} \cdot \mathbf{e}_{\perp}| = y$. We achieve a coarse-grained estimate of $\bar{s}(|\boldsymbol{\theta} \cdot \mathbf{e}_{\perp}|; \varepsilon)$ using two-dimensional basin images by setting $\varepsilon$ equal to the grid spacing. This simplifies the calculation of $\bar{s}(|\boldsymbol{\theta} \cdot \mathbf{e}_{\perp}|; \varepsilon)$ to finding the fraction of points within three consecutive rows that belong to competing basins. For Fig. 4 in the main text and Fig. S6a here, $\varepsilon = 1/128$ and $\varepsilon = 1/1000$, respectively.

We now explain the critical learning period for neural network training, using VGG-12 network training as a representative example. During an early period, which is approximately 100 epochs for VGG-12 network training (Fig. S6c), the transverse component $|\boldsymbol{\theta} \cdot \mathbf{e}_{\perp}|$ remains of roughly constant order of magnitude. At these distances from the attractor, the sensitivity is close to 1, indicating an early period in which the training outcome is highly sensitivity to perturbations. Subsequently, the network converges exponentially to the invariant subspace with a characteristic time of approximately 5 epochs. As the state approaches the invariant subspace, the sensitivity diminishes but does not vanish, even arbitrarily close to the invariant subspace (Fig. S6b). Fundamentally, sensitivity does not vanish because holes of competing basins exist arbitrarily close to the attractor. In contrast, for a non-riddled basin the sensitivity vanishes sufficiently close to the attractor, because proximity alone guarantees convergence. Thus, only the riddling mechanism is consistent with the empirical observation that the sensitivity of the learning process to perturbations is non-vanishing [14].

## Supplementary References


[1] Milnor, J. On the concept of attractor. *Communications in Mathematical Physics* **99**, 177–195 (1985).

[2] Alexander, J., Yorke, J. A., You, Z. & Kan, I. Riddled basins. *International Journal of Bifurcation and Chaos* **2**, 795–813 (1992).

[3] Lai, Y.-C. & Grebogi, C. Riddling of chaotic sets in periodic windows. *Physical Review Letters* **83**, 2926 (1999).

[4] Lai, Y.-C. Pseudo-riddling in chaotic systems. *Physica D: Nonlinear Phenomena* **150**, 1–13 (2001).

[5] Herrmann, L., Granz, M. & Landgraf, T. Chaotic dynamics are intrinsic to neural network training with SGD. *Advances in Neural Information Processing Systems* **35**, 5219–5229 (2022).

[6] Ott, E. & Sommerer, J. C. Blowout bifurcations: the occurrence of riddled basins and on-off intermittency. *Physics Letters A* **188**, 39–47 (1994).

[7] Woltering, M. & Markus, M. Riddled-like basins of transient chaos. *Physical Review Letters* **84**, 630 (2000).

[8] Sohl-Dickstein, J. The boundary of neural network trainability is fractal. *arXiv preprint arXiv:2402.06184* (2024).

[9] Hospedales, T., Antoniou, A., Micaelli, P. & Storkey, A. Meta-learning in neural networks: A survey. *IEEE transactions on pattern analysis and machine intelligence* **44**, 5149–5169 (2021).

[10] Grebogi, C., McDonald, S. W., Ott, E. & Yorke, J. A. Final state sensitivity: an obstruction to predictability. *Physics Letters A* **99**, 415–418 (1983).

[11] Daza, A., Wagemakers, A. & Sanjuán, M. A. Ascertaining when a basin is wada: the merging method. *Scientific Reports* **8**, 9954 (2018).

[12] Kennedy, J. & Yorke, J. A. Basins of wada. *Physica D: Nonlinear Phenomena* **51**, 213–225 (1991).

[13] Achille, A., Rovere, M. & Soatto, S. Critical learning periods in deep neural networks. *International Conference on Learning Representations* (2019).

[14] Summers, C. & Dinneen, M. J. Nondeterminism and instability in neural network optimization. *International Conference on Machine Learning* 9913–9922 (2021).

[15] McDonald, S. W., Grebogi, C., Ott, E. & Yorke, J. A. Fractal basin boundaries. *Physica D: Nonlinear Phenomena* **17**, 125–153 (1985).
